# Supplementary material for: Gaussian Primitives for Deformable Image Registration
Source: arXiv:2406.03394 source file (2024-10-16)
Supplement: Supplementary file 1 [file appendix.tex]

\clearpage
\appendix
\section{Appendix}
\subsection{Ablation Studies}
\paragraph{K Value.} We study the effect of the $K$ value on our Gaussian representation by running experiments with $K$ values ranging from 6 to 40 under the same setting and report the TRE-K curve. As shown in Fig.~\ref{kvalue}, despite achieving promising performance with K value from 15 to 40, GaussianDIR hit a "sweet spot" where the performance peaks before it worsens again. We hypothesize that such a sweet spot exists because too small K will weaken the regularization effectiveness and too large K will discourage complex deformation.

\paragraph{Prune Randomly.} To validate the robustness of our method, we randomly prune Gaussians after the optimization process and evaluate the TRE on the DIR-Lab dataset. As shown in Fig.~\ref{random_prune}, pruning up to $5\%$ of the Gaussians does not significantly impact performance, and GaussianDIR still surpasses IDIR and DL-based methods. 

\begin{figure}[htbp]
\begin{minipage}{0.48\linewidth} 
    \centering 
    \includegraphics[width=\textwidth]{images/k-value.pdf} 
    \vspace{-0.4em}
    \subcaption{Landmark error for different $K$ values.} 
    \label{kvalue} 
\end{minipage}
\begin{minipage}{0.48\linewidth} 
    \centering 
    \includegraphics[width=\textwidth]{images/randomprune.pdf}  
    \vspace{-0.4em}
    \subcaption{Landmark error for different pruning ratios.} 
    \label{random_prune} 
\end{minipage}
\caption{Landmark error, averaged across 10 cases, is assessed for different values of K and pruning ratios. Each square's size represents the standard deviation of the respective data point. Larger squares denote higher standard deviations, indicating greater variability in the data.}
\end{figure}
